# Supplementary material for: Alternating Bias Assisted Annealing of Amorphous Oxide Tunnel Junctions
Source: arXiv:2401.07415 source file (2024-08-16)
Supplement: Supplementary file 1 [file ABAA_Supplmentary.tex]

\documentclass{article}
\usepackage{blindtext}
\usepackage[
backend=biber,
style=phys,
]{biblatex}
\usepackage{graphicx}% Include figure files
\usepackage{dcolumn}% Align table columns on decimal point
\usepackage{bm}% bold math
\usepackage{float}
\usepackage{array}
\usepackage{textcomp}
\usepackage{physics}
\usepackage[dvipsnames]{xcolor}
\usepackage{multirow}
\usepackage{booktabs}
\usepackage{upgreek}
\usepackage{xr}
\usepackage{cleveref}
\usepackage{tabularx}
\usepackage{amsmath}
\usepackage{appendix}
\usepackage{gensymb}
\usepackage{fixltx2e}
\addbibresource{VIA.bib} 
\usepackage{xcolor}

\makeatletter
\DeclareRobustCommand{\change}{%
  \@bsphack
  \leavevmode
  \color{black}%
  %\normalcolor
  \@esphack
}
\DeclareRobustCommand{\stopchange}{%
  \@bsphack
  \normalcolor
  \@esphack
}
\makeatother

\title{Supplementary Information for Alternating Bias Assisted Annealing of Amorphous Oxide Tunnel Junctions}
\author{D. P.~Pappas$^1$, M.~Field$^1$,C. Kopas$^1$, J. A.~Howard$^1$, X.~Wang$^1$, E.~Lachman$^1$, \\Lin~Zhou$^{2,3}$, insu~Oh$^{2,3}$, K. Yadavalli$^1$,   Alysson Gold$^1$,  G.M. Stiehl, \\E. A.~Sete$^1$, A. Bestwick$^1$, M.J. Kramer$^{2,3}$, J. Y. ~Mutus$^1$\\$^1$\textit{Rigetti Computing, 775 Heinz Avenue, Berkeley, CA 94710, USA}\\$^2$\textit{Ames National Laboratory, Ames, IA 50011, USA}\\$^3$\textit{Department of Materials Science and Engineering,}\\ \textit{ Iowa State University, Ames, IA 50011, USA}}

\date{\today}

\begin{document}
\maketitle

\section*{Note 1: Dependence of ABAA on Junction Size} 
Typically two different-size junctions, connected in parallel, are used in order to make an asymmetric SQUID for qubit tunability. For these devices, it is important that the ABAA process works for both junctions in a similar manner.   This hinges on the idea that the process is voltage-driven. To establish this, the ABAA process was conducted  on an ensemble of test junctions of different areas, plotted in 
Figure~\ref{Fig_ABAAvsArea}. The data was taken for nominally identical parameters, i.e. voltage, pulse duration, and pulse number. \change We see \stopchange that the ABAA process has a slight negative dependence on area of 31$\pm$8 $\ohm / \mu$m$^2$.    

\section*{Note 2: Extracting Junction and Qubit Parameters}
Critical currents were extracted using the transmon relations from Koch, et al.\cite{koch2007charge}. Specifically, the  anharmonicity, $\alpha=\omega_{01}-\omega{12}\approx E_C$, and frequency, $\omega_{01}\approx \sqrt{8E_cE_J}$, 
relationships were used to find $I_0=2\pi E_J/\Phi_0$. The results of this are shown in Figure~\ref{Fig:I_0}

\section*{Note 3: Success Statistics of ABAA Process}
\subsection*{Note 3.1:Yield from initial tests} For the initial measurements of frequency tuning, coherence and TLS tests, we selected 5 equivalent chips from a general-purpose test wafer for junction process development. Due to the nature of the test wafer, there are typically dropouts that are not necessarily related to the ABAA process. On this wafer, each chip had 16 qubits; 14 flux-tunable  and two fixed qubits (30 junctions on each chip). Two chips were control devices with no ABAA process (unprocessed). Of the three remaining chips, all were processed to 80 $\degree$C, while qubits on one and a half chips  were processed with ABAA. This corresponds to 24 qubits, i.e. 43 junctions. Among these processed qubits, 3 failed to a short circuit and 6 others lost tunability, hence only 9 junctions failed. This translates to a success yield of 79\%.

Based on the fact that this was a process-test wafer, it was likely that these failures are attributable to lithography, the other process steps, and imaging issues. These included various exposure tests, electrostatic issues due to extra handling, and SEM-induced imaging faults that are not present for standard wafers. This is consistent with the fact that some of the control-group devices failed. 

\subsection*{Note 3.2: Extended Tests of ABAA}
 In order to isolate the yield of the ABAA process, it was optimized using ranges of ABAA parameters described in the main text and \change Note 1. These were \stopchange applied to wafers that were only exposed to standard processing. In this extended study, a total of 1034 ABAA-treated tunable-qubits and tunable-couplers with SQUID-loops (i.e. 2 junctions each, so 2068 junctions) were made, and 200 of these qubits have been measured at 10 mK to date. Of the 2068 junctions, we observed a resistance yield of 98.9$\pm 0.4$\%. Of the measured devices, we found a success rate of 98.5\%. This gives a net yield of 97.4$\pm0.4$\%. 

\section*{Note 4: Qubit Spectroscopy} 
Strongly coupled TLS were studied using qubit spectroscopy of the tunable qubits across the flux period.  While no strongly coupled TLS were observed in qubits treated by ABAA, in the unprocessed qubits, there were an average of 0.7 TLS/GHz seen in a 21-qubit ensemble with a 10 GHz total tunable range. Based on this, we would have expected to see $\sim$ 3 - 4 TLS in the 9-qubit, 5.4 GHz tunable range of ABAA trimmed junctions.
An example of a strongly-coupled TLS in an untreated qubit is shown in Fig~\ref{Fig:StronglyCoupledTLS},  with the avoided level fitting shown in Fig.~\ref{Fig:AvoidedCrossingTLS}.

For comparison, we show spectroscopy from nine example ABAA-treated qubits in Fig.~\ref{Fig:QubitSpectroscopyFullChip}. In addition, we show a zoomed-in version of Fig.4(a) from the paper in Fig.\ref{Fig:ZoomedFeatures}. While there are small features in the spectroscopy observed in this ABAA qubit, careful analysis shows that they are due to couplings with other qubits on the chip. The salient characteristic of these features is that there is no distinct splitting observed, as shown above, that would tie these to strongly coupled TLSs in the junction.

\section*{Note 5: Example of Qubit Stability} 
The frequency of one ABAA-treated qubit was measured over an extended time to evaluate the stability. The mean qubit frequency over the full duration of measurements, three days in total, is 4,280.56 ± 0.001 MHz. For the subset of the data shown in Fig.~\ref{Fig:TimeTrace}, two protocols were used. The first protocol, i.e. "slow" measurements, averaged the Ramsey oscillation frequency for 15-minute intervals, while the "fast" measurements used a much shorter, 15-second averaging interval. This was done to check if there were fast jumps that were not being resolved in the slow measurements. The standard deviation over the slow measurement dataset is 0.028 MHz, and it scaled as expected for the fast measurements. No fast jumps in the frequency were observed. 

\section*{Note 6: Qubit Loss} 
 A Tabulation of the ABAA-treated qubit coherence values, from the data (Manuscript Figure 5), are shown in Table~\ref{decoherence}   and  the values for the loss of qubits from same devices are shown in Figure~\ref{Fig:Loss}. The number of measured qubits in the unprocessed data set is $n_{\rm qubit}=30$, the  $80\degree$C anneal-only set has $n_{\rm qubit}=22$, and the ABAA tuned set has $n_{\rm qubit}=21$.
\begin{table}[h]
\begin{tabular}{c|c|c|c} 
 \hline
 \hline
 Qubit Coherence & $T_1$ ($\mu$s) & $T_2^*$ ($\mu$s) & $T_{\phi}$ ($\mu$s) \\ 
 \hline
 ABAA treated & $28.4 \pm 8.7 $ & $34.1 \pm 10.6$ & $62.5 \pm 23.1$ \\ 
 80~$\degree$C annealed & 20.9 $\pm$ 4.6 & 29.0 $\pm$ 12.7 & 37.9 $\pm$ 39.9 \\
 Unprocessed & $19.5 \pm 5.0 $ & $22.7 \pm 12.3$ & $41.4 \pm 45.1 $ \\
 \hline
 \end{tabular}\\
\caption{\\Title: Coherence times measured for qubits in this study.\\
Legend: Three groups of qubits were studied. The first row shows coherence times for qubits that were ABAA treated at 80~$\degree$~C, the second row shows coherences for qubits that were only annealed at 80~$\degree$~C, and the third row shows results for unprocessed qubits. The error bars are $1\sigma$ standard deviations.}
\label{decoherence}
 \end{table} 

\section*{Note 7: TEM Characterization}
Secondary electron images for the Josephson junction surface were acquired using a scanning electron microscope (SEM) (Helios, Thermo Fisher Scientific Ltd.) at 2 kV. Transmission electron microscope (TEM) samples were prepared by a focused ion beam instrument with a gas injection system (Helios, Thermo Fisher Scientific Ltd.). The TEM samples were thinned to electron beam transparency by a Ga$^{+}$ ion beam from 30 to 2 kV. The TEM samples were investigated by an aberration-corrected TEM (Titan Cube, Thermo Fisher Scientific Ltd.) at 200 kV. A high-angle annular dark-field (HAADF) detector was used for dark-field imaging in scanning TEM (STEM) mode with a convergent semi-angle and a collection semi-angle of 18 m rad and 74-200 m rad, respectively. Energy-dispersive X-ray spectroscopy (EDS) and electron energy-loss spectroscopy (EELS) studies were carried out with probe currents of 250 nA and 50 nA, respectively. Dual EELS was performed to acquire all-electron energy-loss (ELL) spectra. The plural scattering effect of all the raw ELL spectra was removed via Fourier-ratio deconvolution. 

The EELS data were taken from a typical thin spot of the barrier. We do not have EELS data from the areas around grain boundary regions, but from earlier work, we observe that the oxides are significantly thicker in those regions, and hence are not expected to participate in the tunneling process.

\section*{Note 8: Finding the Voltage Range for ABAA}\label{VoltageRange}
A relevant concern when probing and applying voltages to junctions is the fact that they are highly sensitive. In particular, in this case, they either revert irreversibly to a short or open when excessive voltage is applied. On the other hand, it is clear that the voltages present during oxidation do not generate these changes. Therefore, we used voltages in the range below the typical break-down voltages for these junctions and above the typical Mott voltage. In order to establish the former and find the latter, breakdown experiments were conducted on junctions and literature was searched. The results of these studies are shown in Figure~\ref{Fig:ABAA_Voltage_Range}. The green bar shows the range available where it is less than the breakdown and greater than the typical Mott voltage generated at room temperature and about $1\times10^{-5}$ Torr. In general, we find that the ABAA process works reliably in the green voltage range shown spanning  \change Figure~\ref{Fig:ABAA_Voltage_Range}(a) to 9(b), with the ABAA-induced \stopchange resistance tending to increase faster with higher voltage. This voltage range will likely depend on the specifics of the ionic material used for the junctions as well as the morphology, i.e. thickness, roughness, and composition.

\begin{figure}[h]
\includegraphics[trim={0 0 0 0},clip,width=\columnwidth]{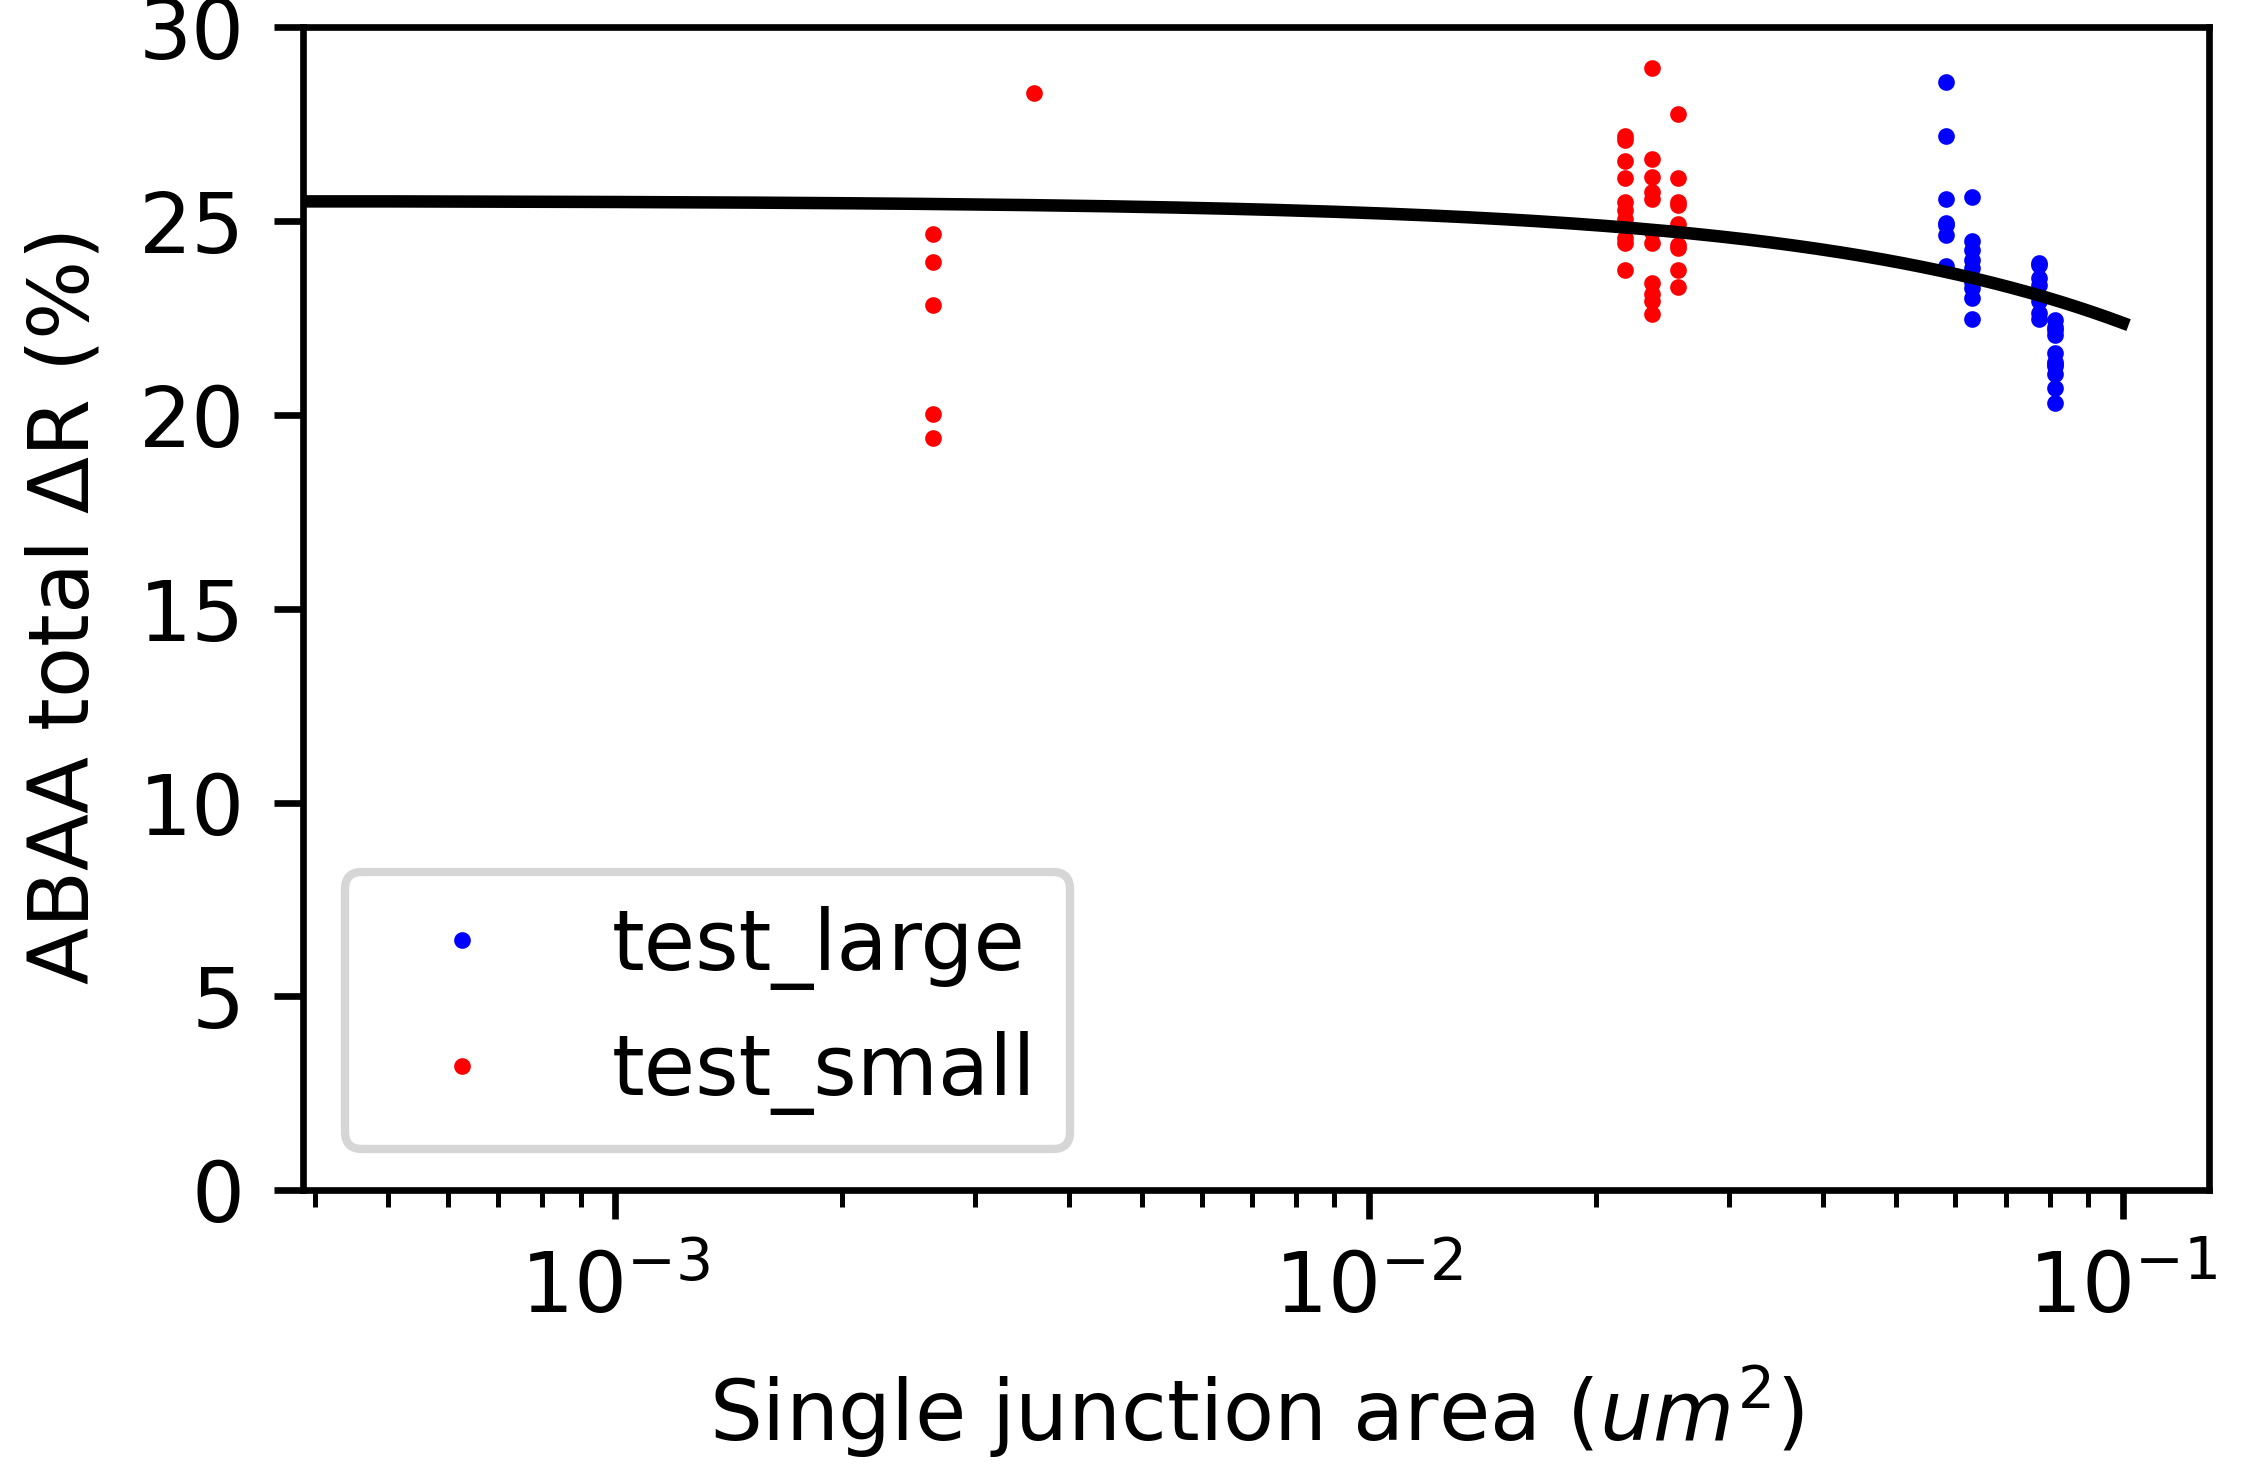}
  \caption{\\Title: Dependence of ABAA trimming effect on junction size\\
  Legend: The resistance change due to ABAA of various sized junctions with a linear fit, $y=ax+b$ where $a=-31\pm8$ and $b=25.5\pm0.4$ for this particular wafer and fabrication process. The x-axis is plotted as a log scale so the sizes of the small and large junctions can be resolved.}
\label{Fig_ABAAvsArea}
\end{figure}

\begin{figure}[h]
\includegraphics[width=4in]{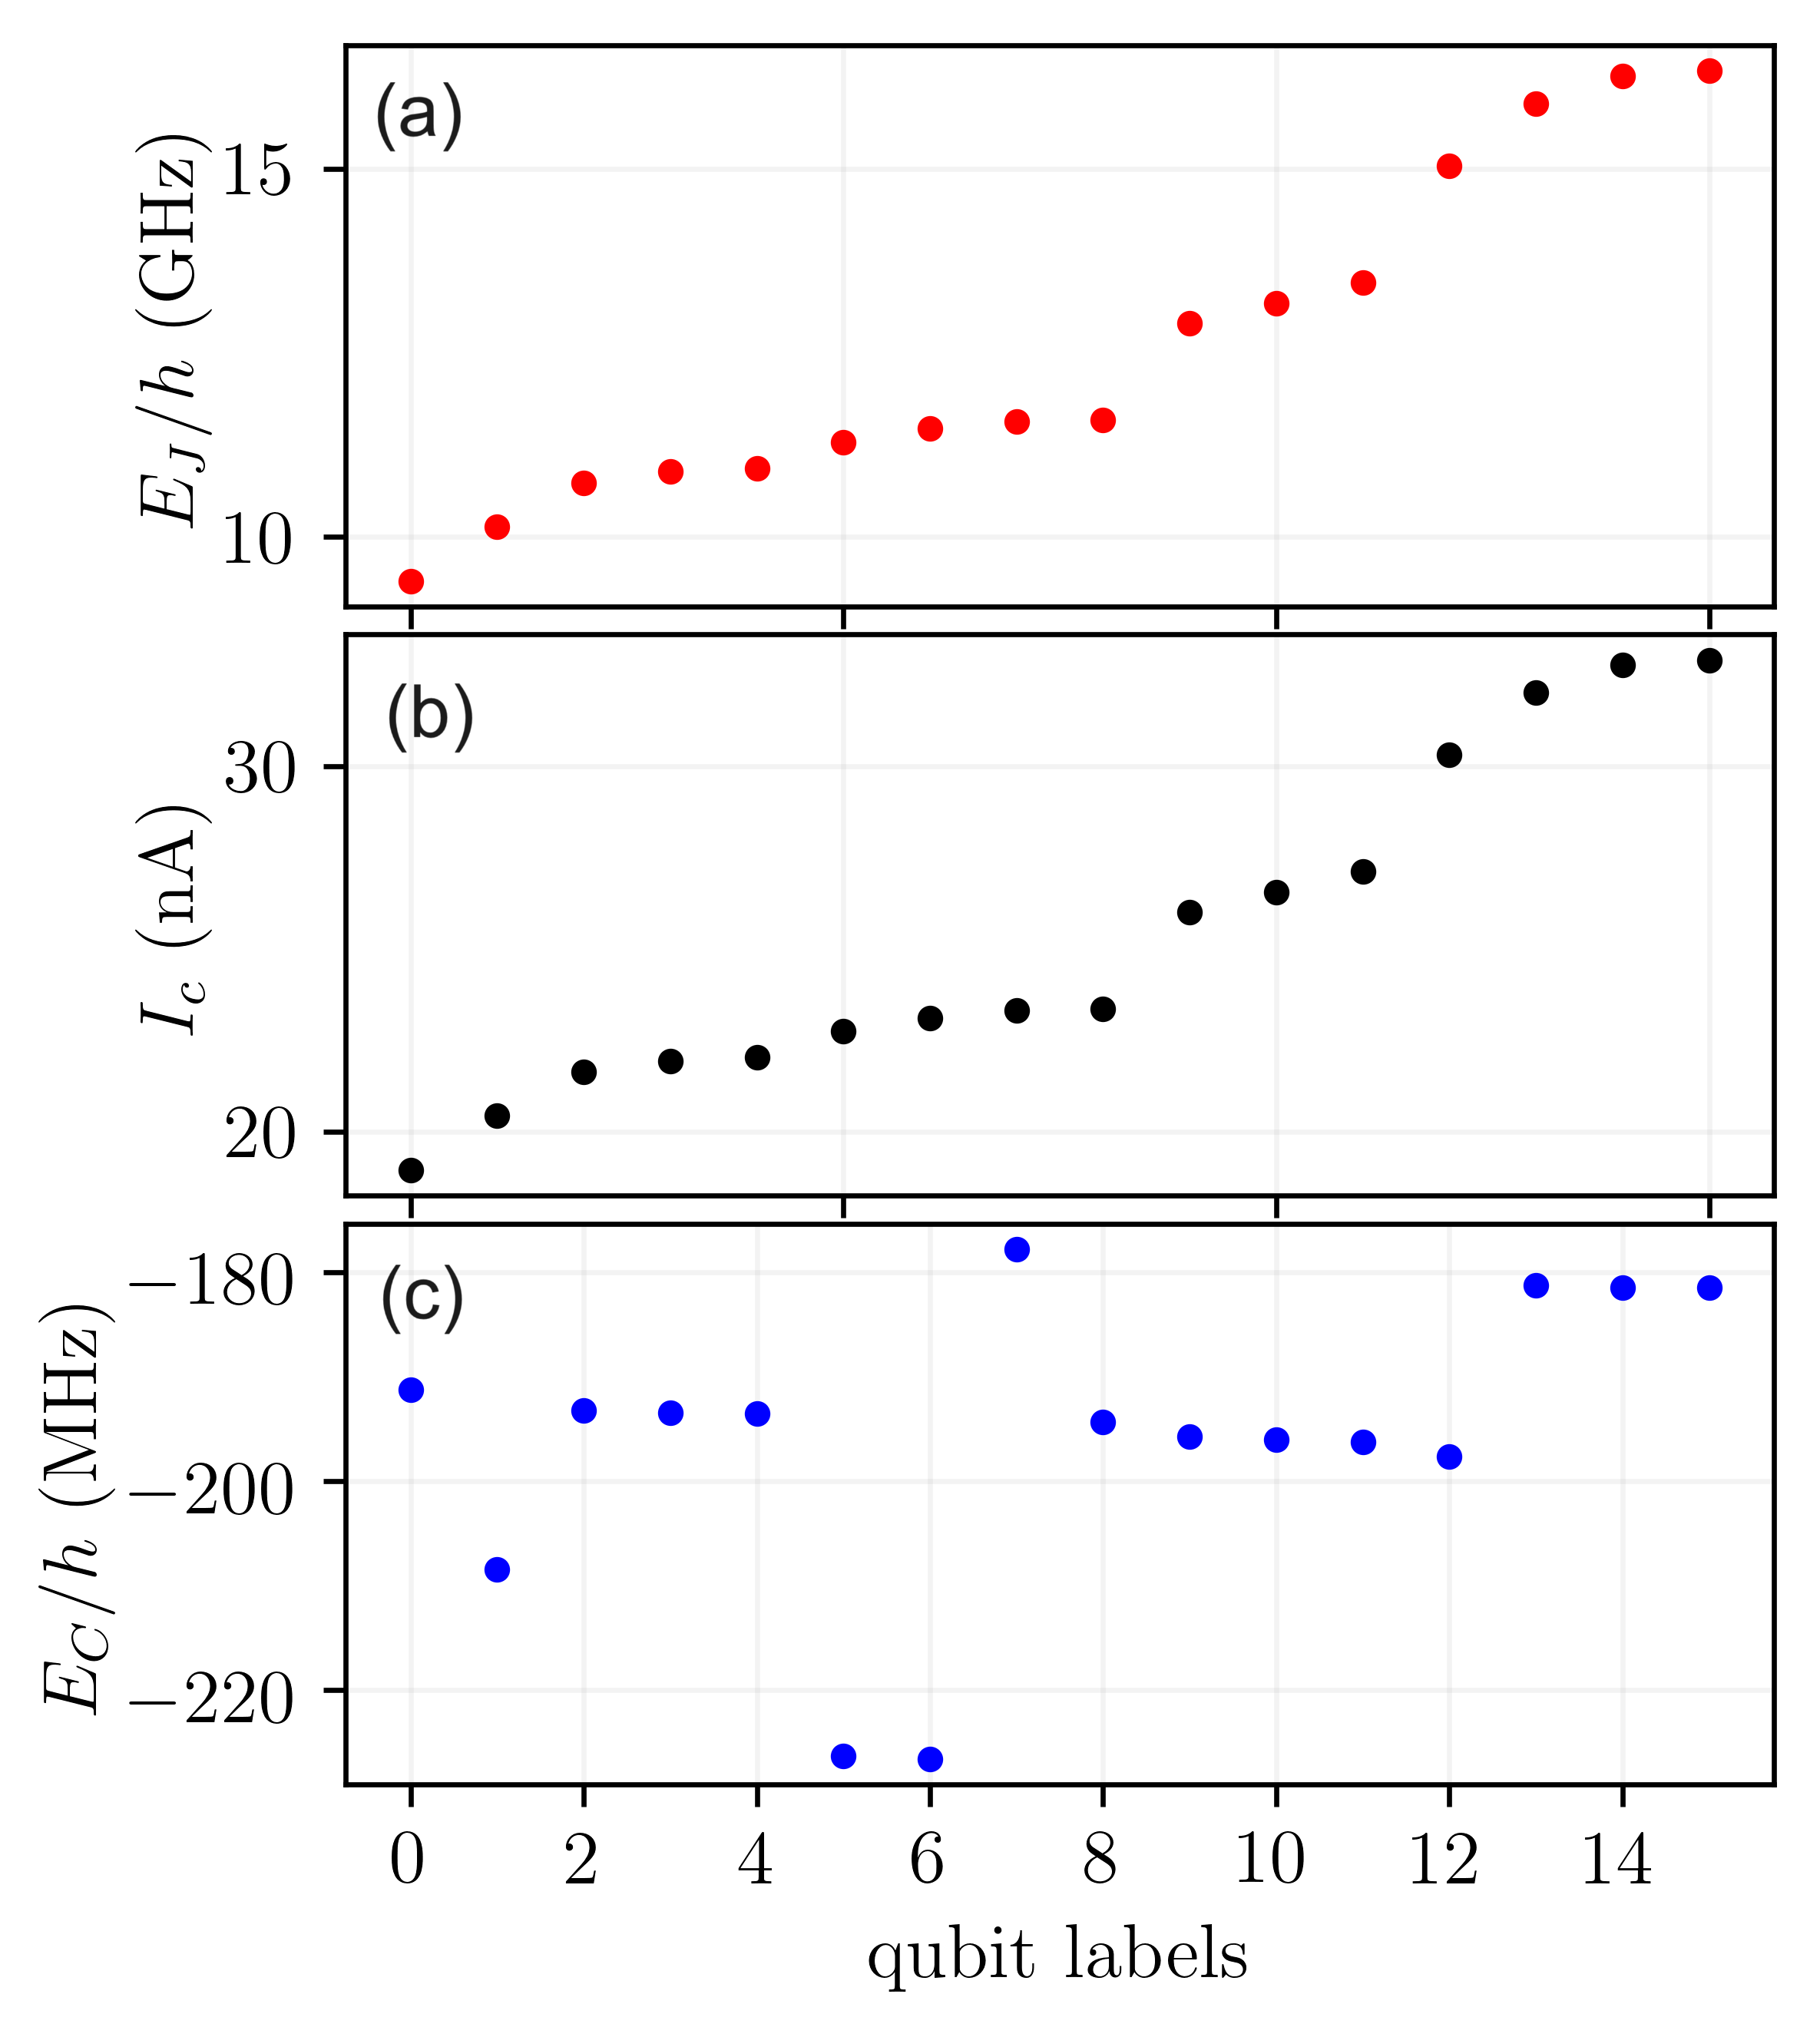}
\caption{\\Title: Qubit parameters from devices in study.\\
Legend: Panels (a)-(c)show the values of $E_J$, $I_c$, and $E_C$, respectively, extracted out of data taken from 15 ABAA-treated qubits.}
\label{Fig:I_0}
\end{figure}

\begin{figure}[h]
\includegraphics[trim={0 0 0 0.7in},clip,width=\columnwidth]{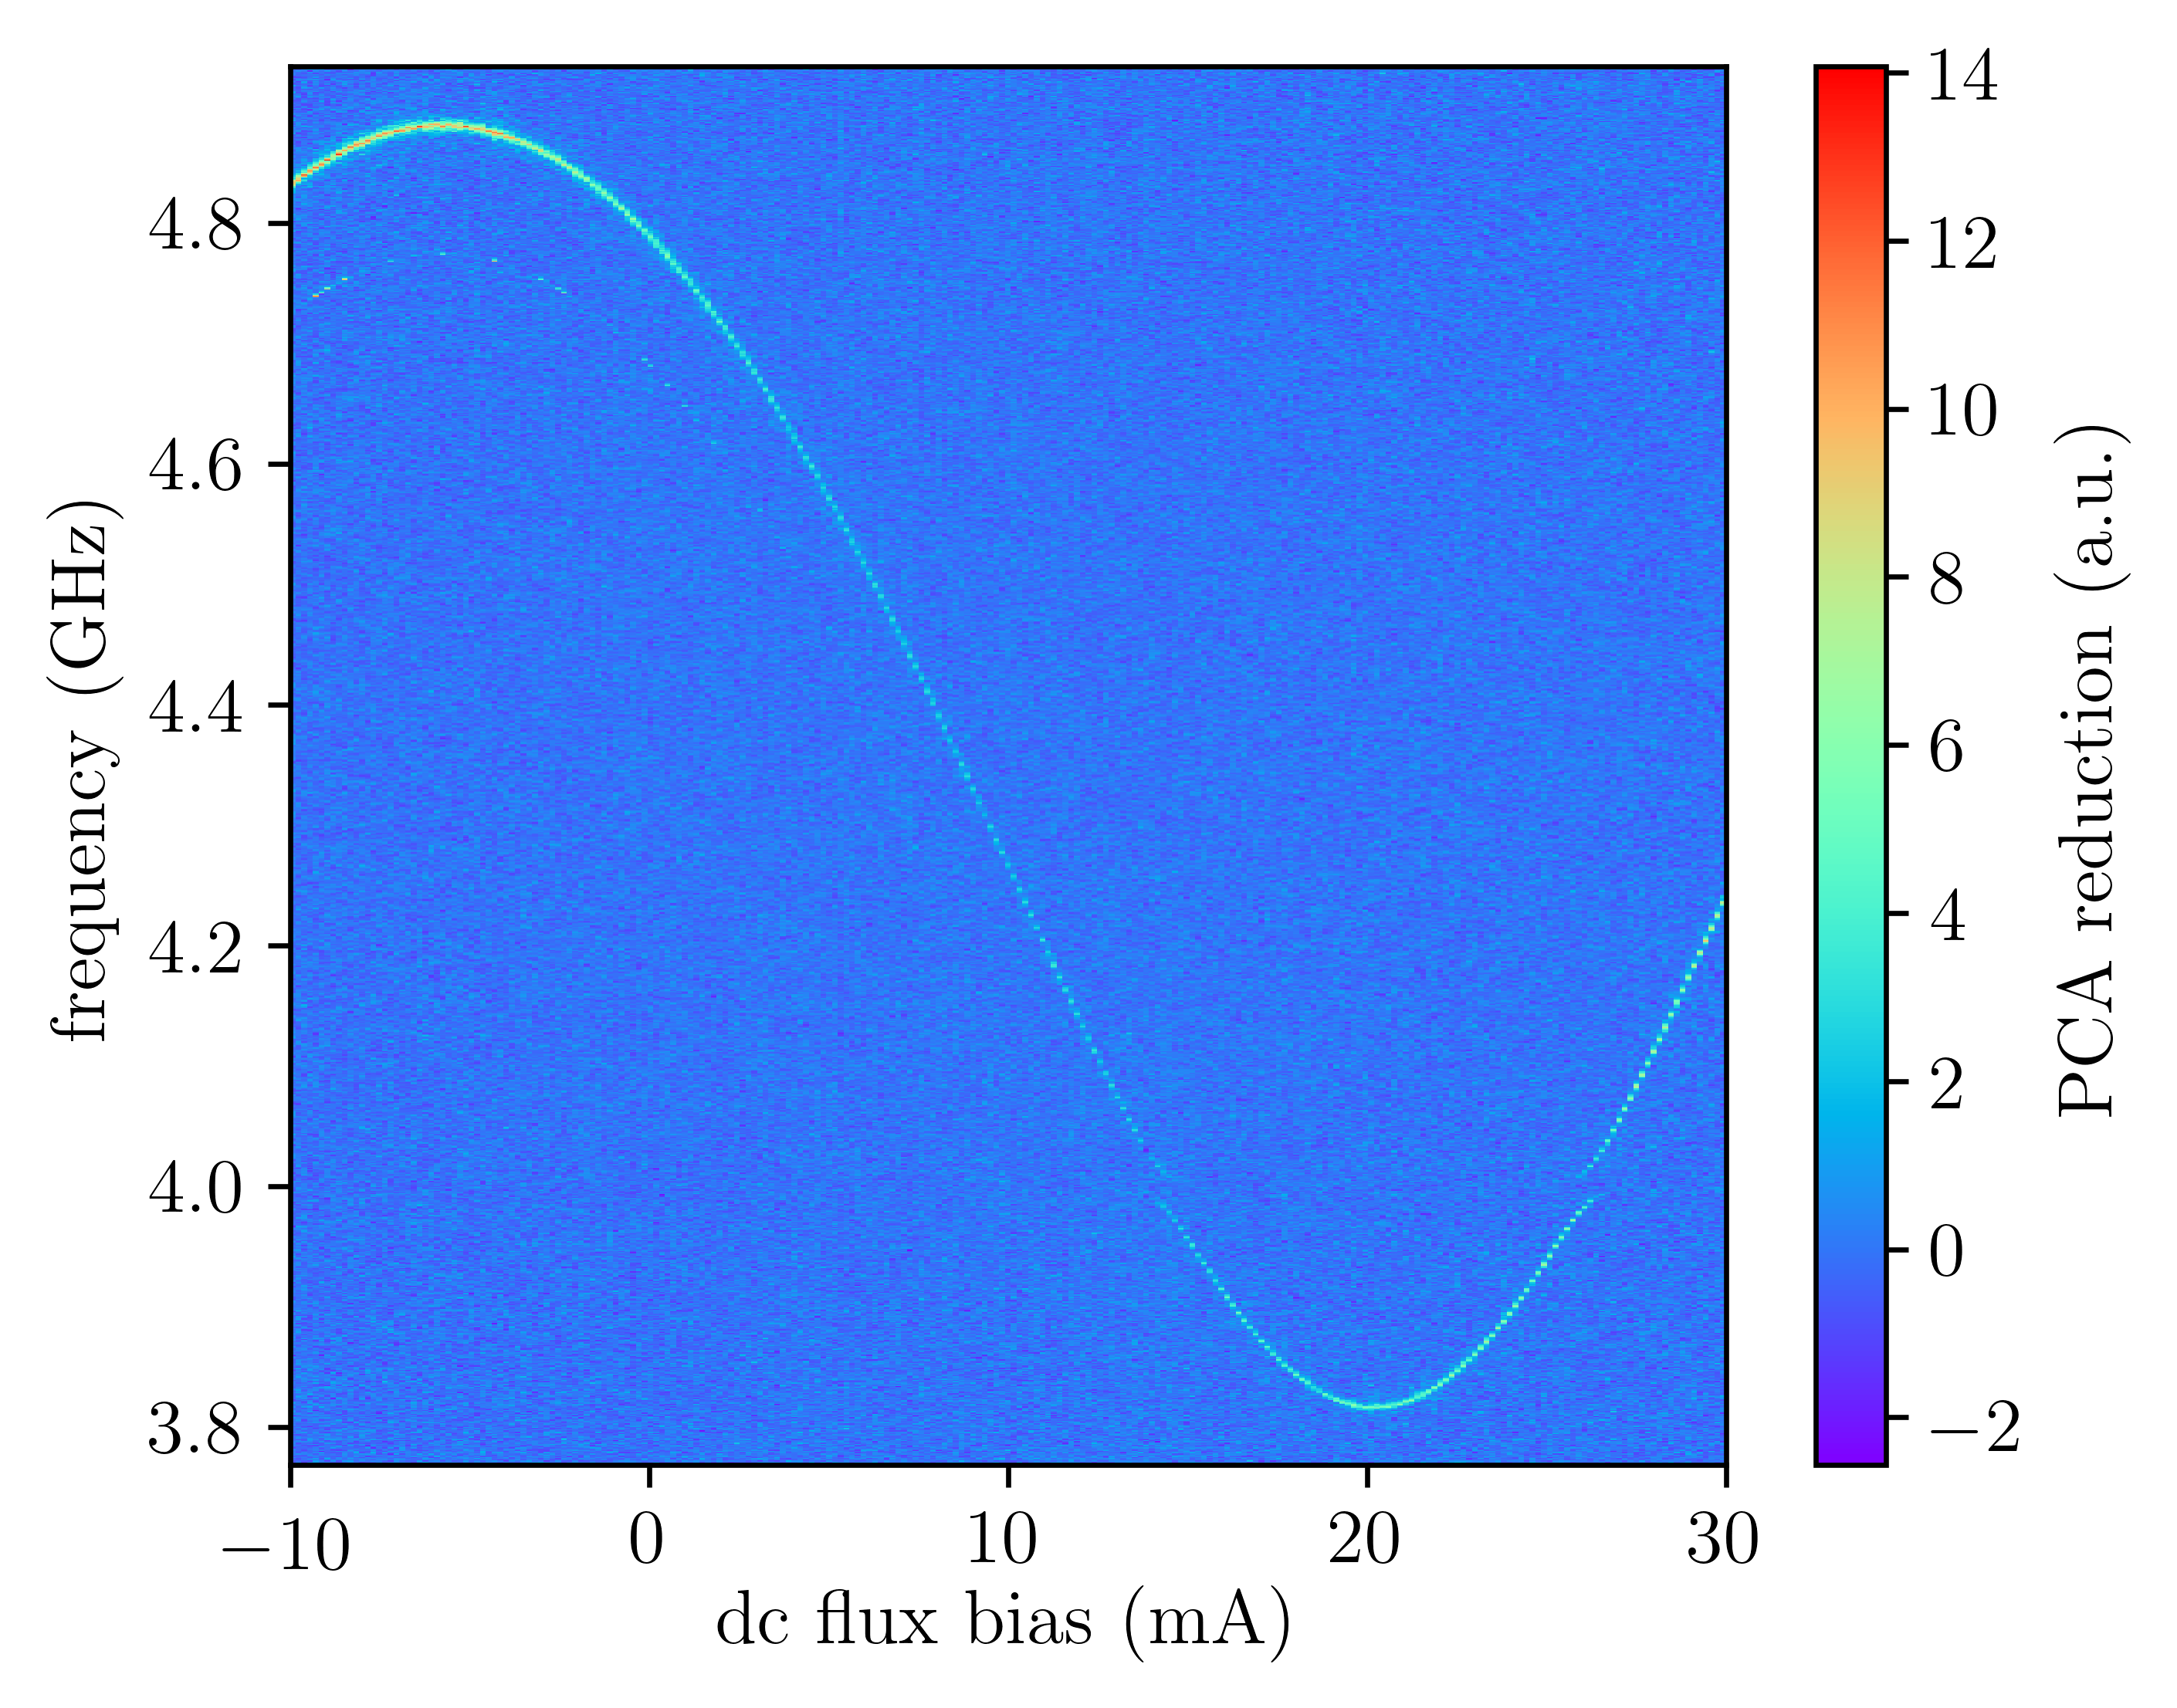}
\caption{\\Title: Example of strongly coupled TLSS in qubit spectroscopy\\
Legend: Data from an untreated qubit illustrating a strongly coupled TLS near 4 GHz.}
\label{Fig:StronglyCoupledTLS}
\end{figure}

\begin{figure}[h]
\includegraphics[width=\columnwidth]{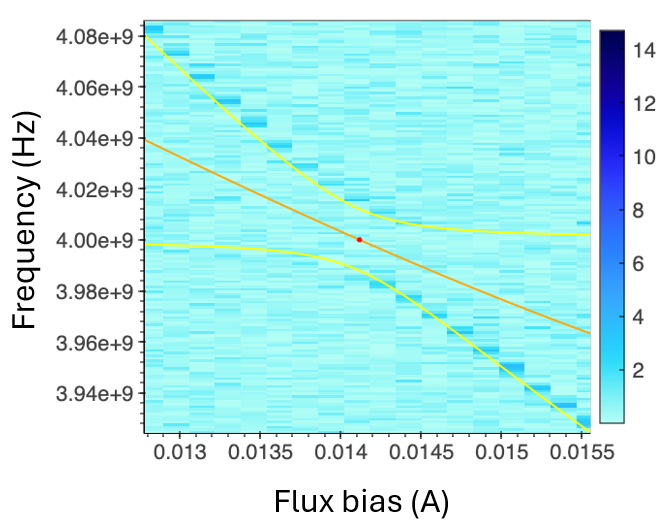}
\caption{\\Title: Zoomed-in example of strongly coupled TLS\\
Legend: Spectroscopic data from and untreated qubit illustrating the spectroscopic behavior of a strongly coupled TLS, fit to the avoided level crossing in Fig.~\ref{Fig:StronglyCoupledTLS}}
\label{Fig:AvoidedCrossingTLS}
\end{figure}

\begin{figure}[h]
\includegraphics[width=4in]{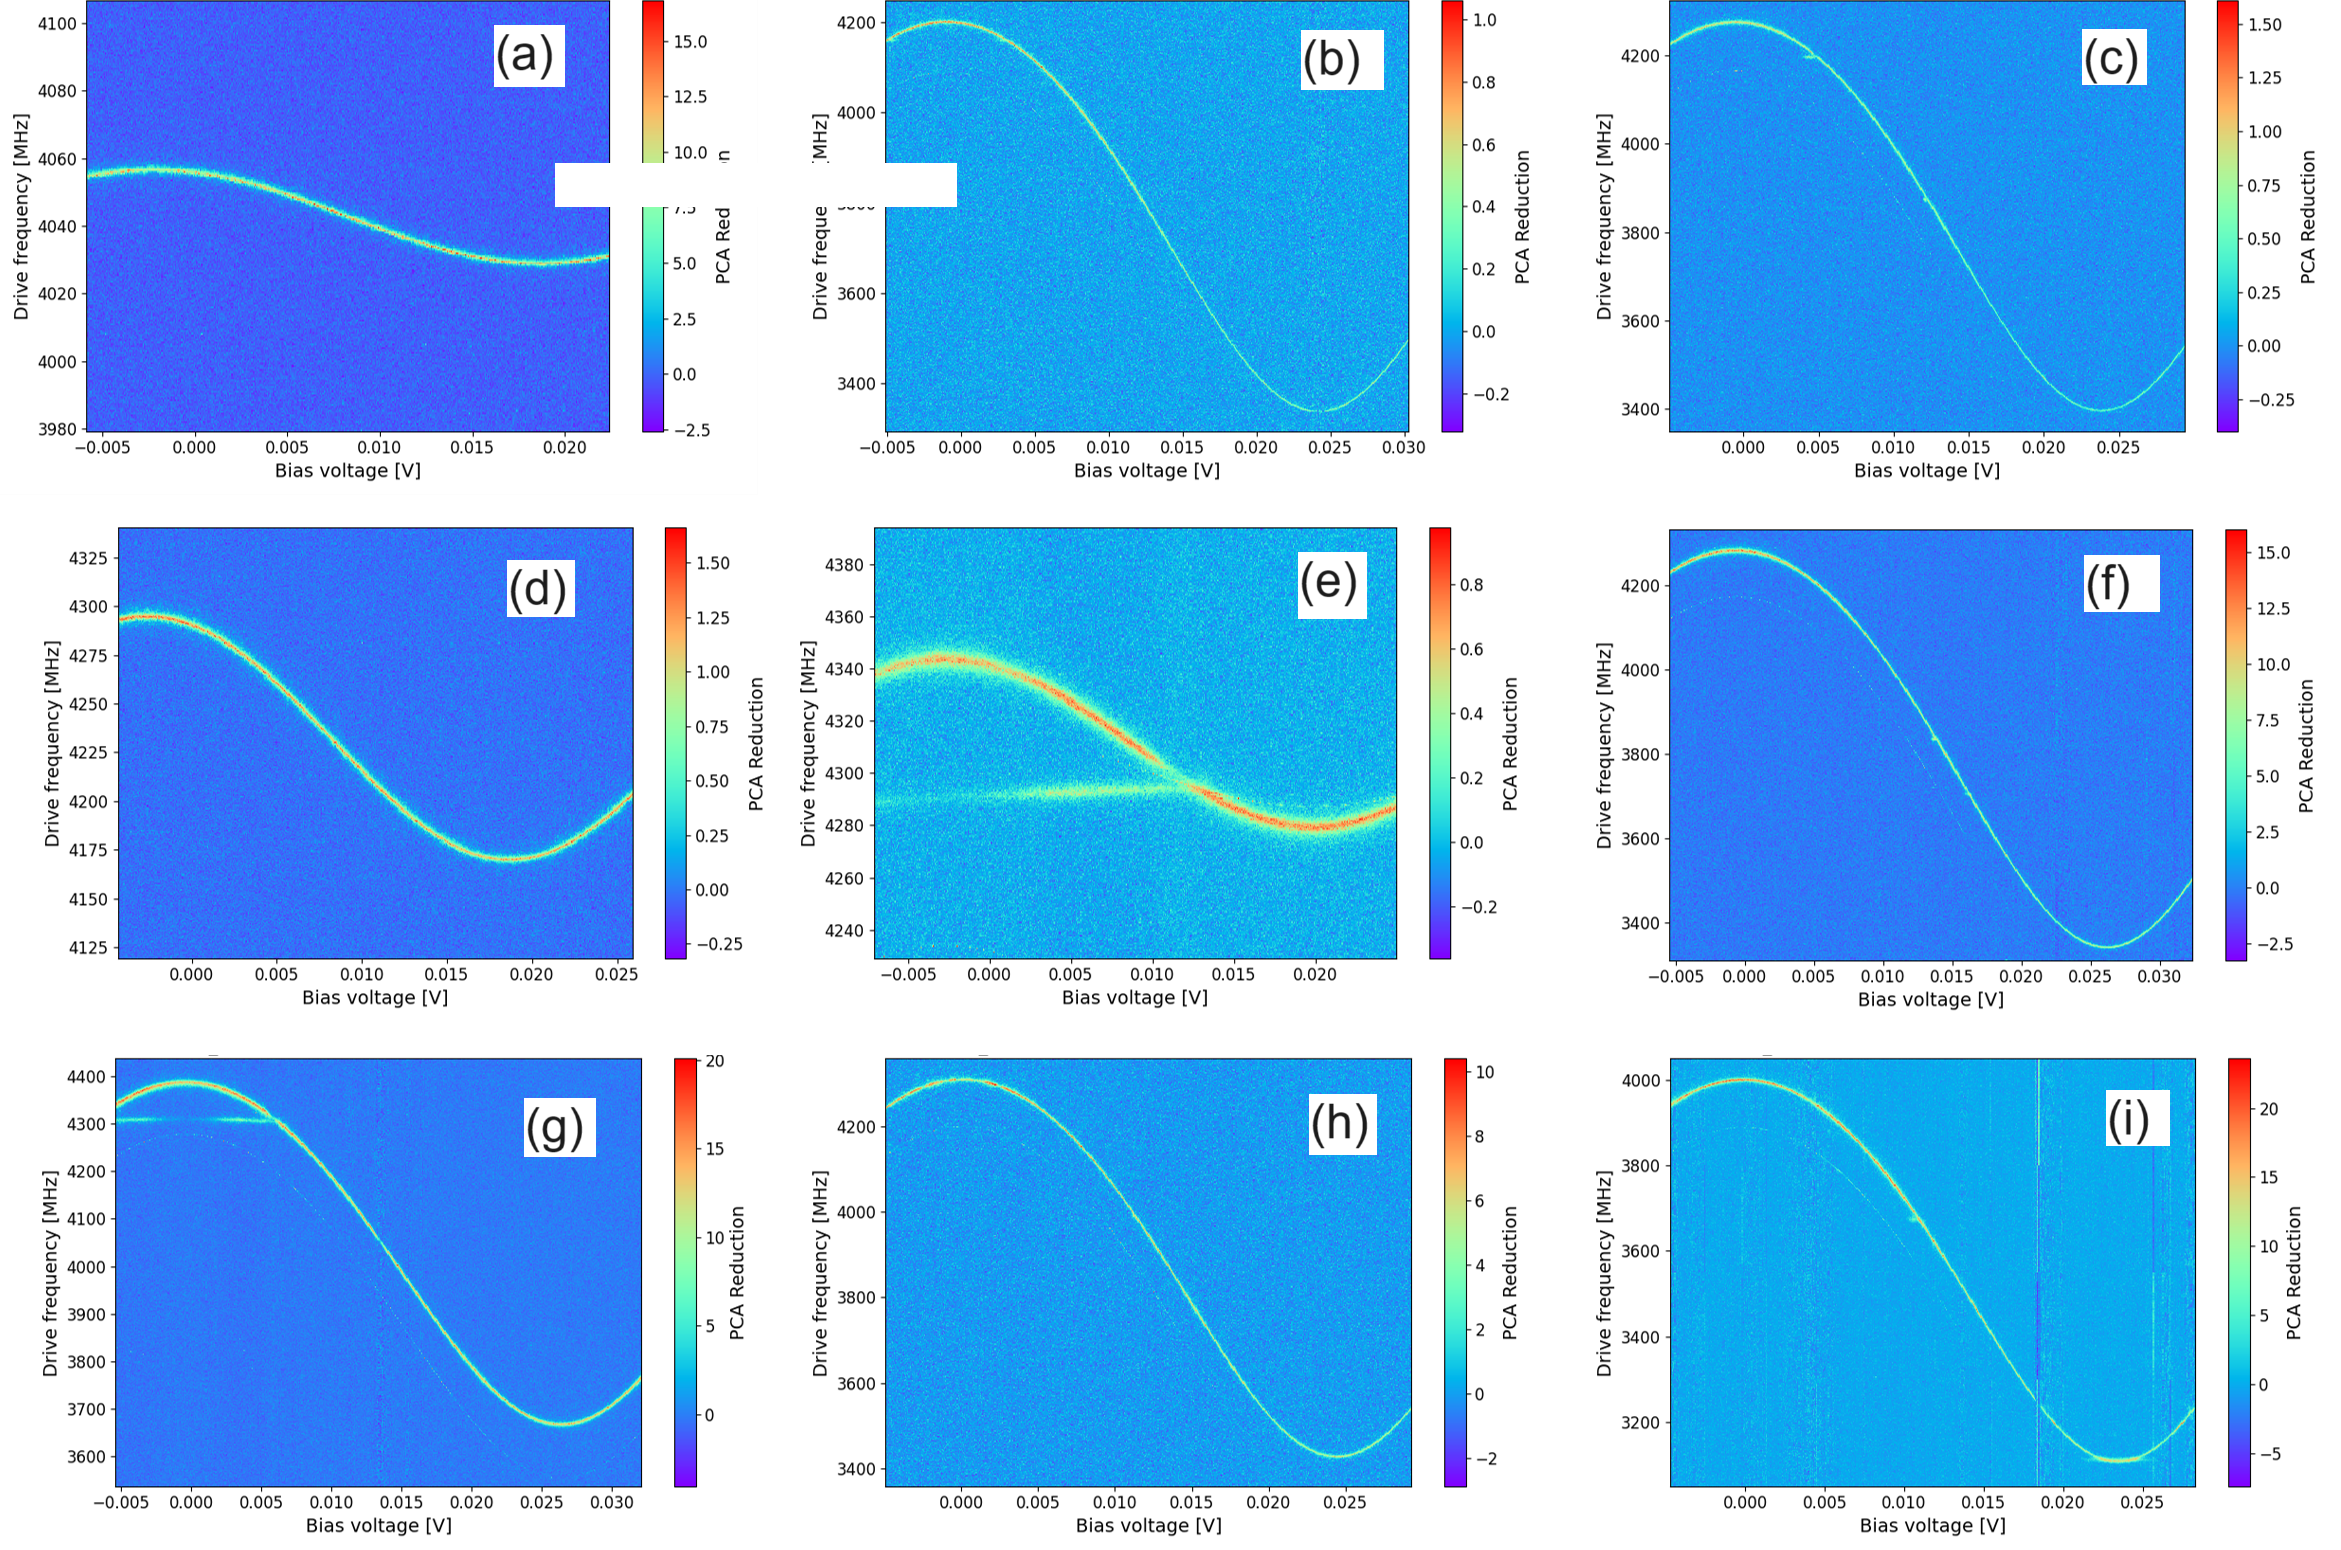}
\caption{\\Title: Qubit spectroscopy from devices with ABAA-treated junctions.\\
Legend: Panels (a)-(i) shows the individual qubit spectroscopy from each of the nine devices with junctions treated with ABAA. The data shows no strongly-coupled splittings. Horizontal lines in the spectra are correlated with classical cross-talk other components on the chip.}
\label{Fig:QubitSpectroscopyFullChip}
\end{figure}

\begin{figure}[h]
\includegraphics[trim={0 0 0 0.25in},clip,width=\columnwidth]{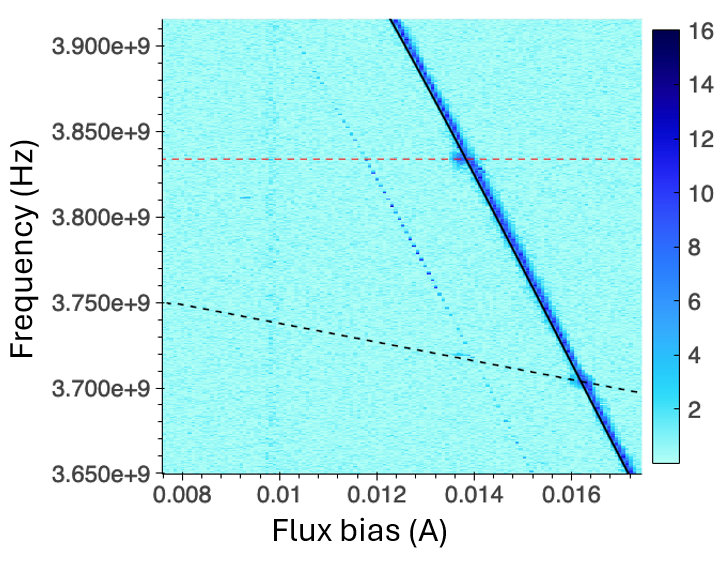}
\caption{\\Title: Example of ABAA-treated qubit without splittings\\
Legend: Zoomed in region of data from an ABAA-tuned qubit showing faint features. The red dashed line is a nearest neighbor that is a fixed qubit, and the black dashed line is a nearby tunable qubit. The $f_{02}/2$ trace is visible \~0.11 GHz below the $f_{01}.$ line}
\label{Fig:ZoomedFeatures}
\end{figure}

\begin{figure}[h]
\includegraphics[trim={0 0 0 0},clip,width=\columnwidth]{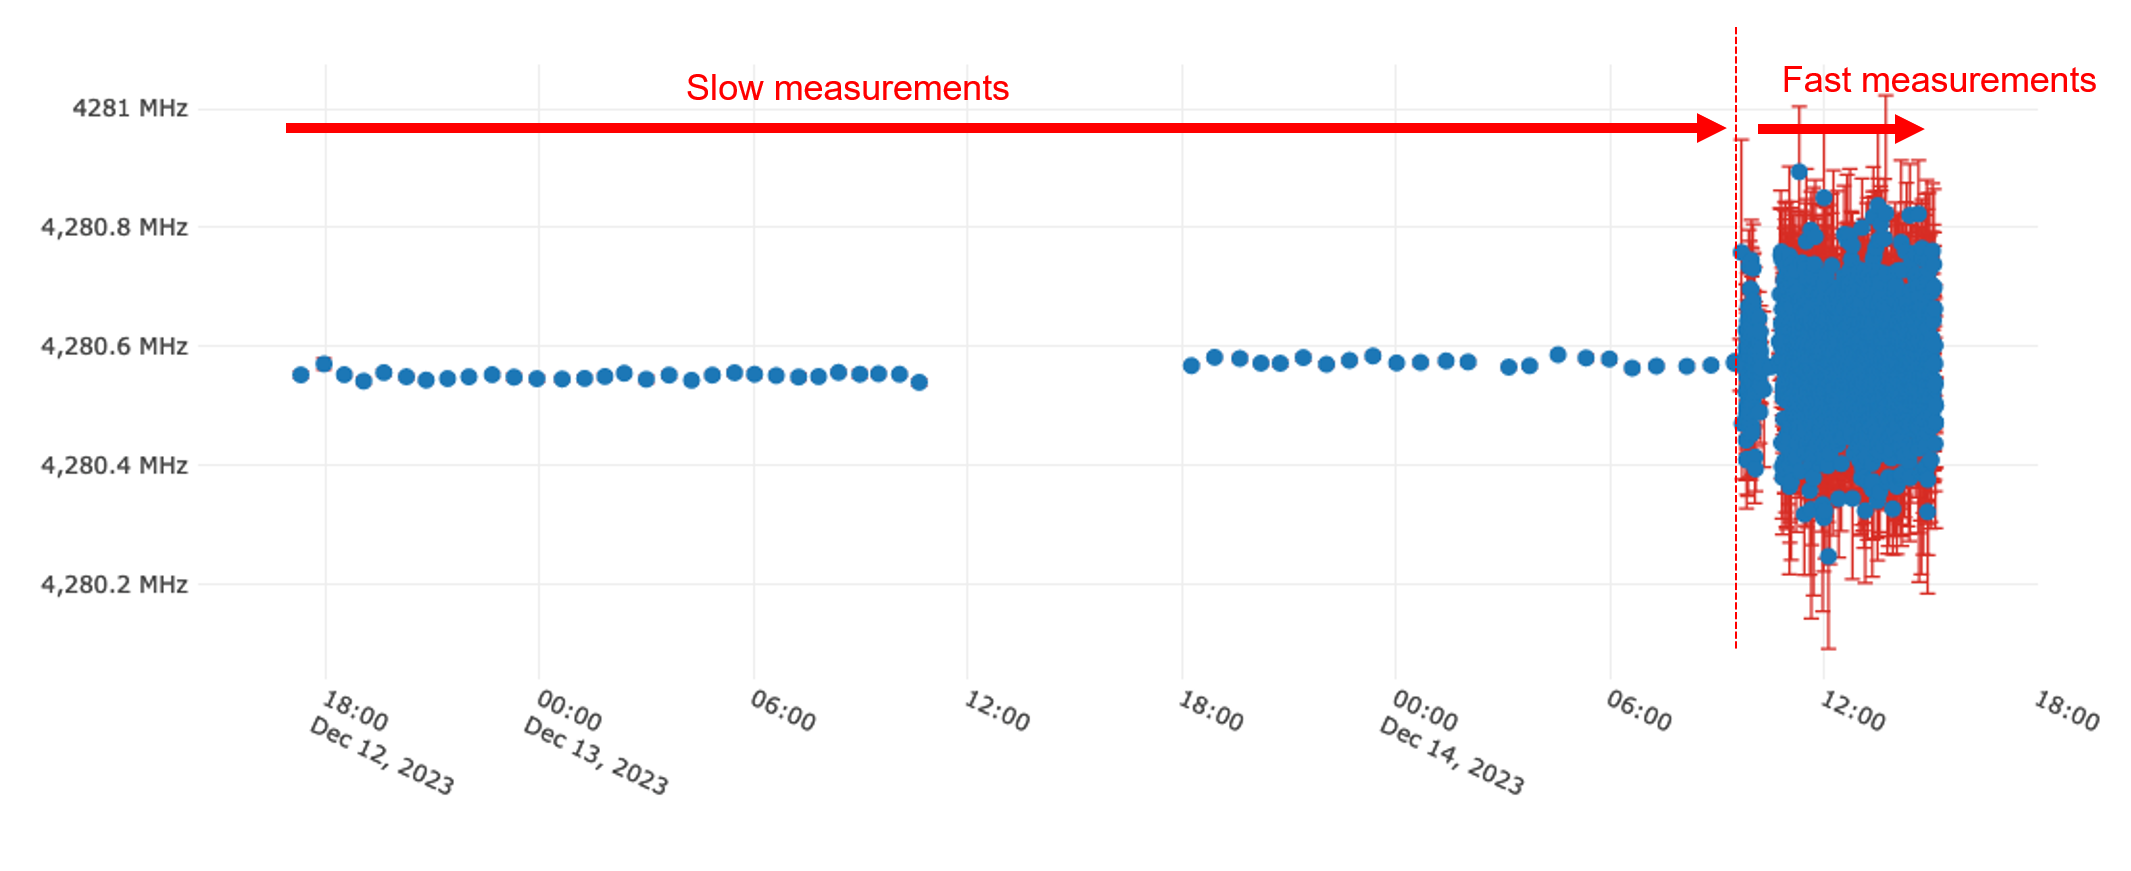}
\caption{\\Title: Example of qubit stability.\\
Legend: Time trace of a single qubit's frequency over an interval of about 46 hours.}
\label{Fig:TimeTrace}
\end{figure}

\begin{figure}[h]
\includegraphics[width=4in]{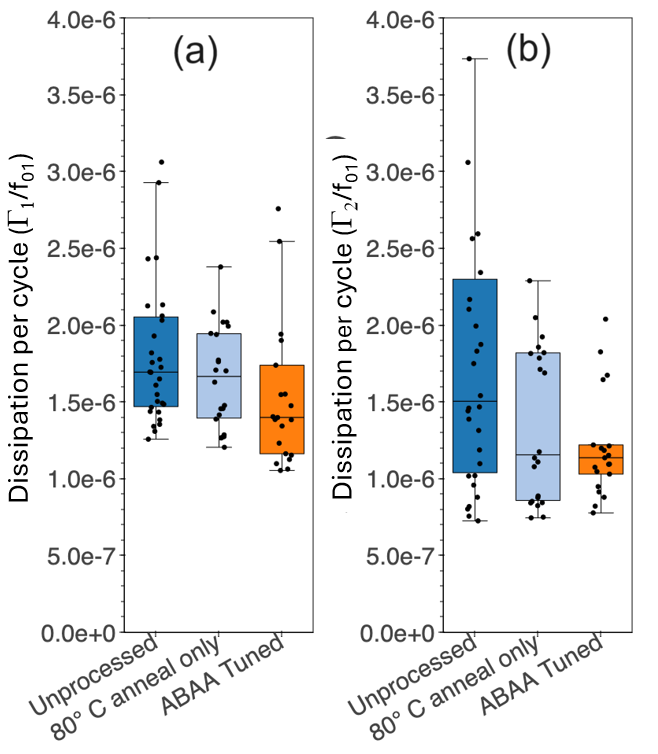}
\caption{\\Title: Loss plots of ensemble of multiple qubits, from main paper's coherence data. \\
Legend: Data converted to loss using qubit frequency and quality factor definition. Panel (a) shows the energy loss rate, while Panel (b) shows the decoherence rate. High standard deviation points are not shown, but are included in the standard deviation. The filled boxes error boxes span the 1st and 3rd quartile of the data uncertainty, while the whiskers mark the furthest datum within the $1.5\times$ the interquartile range past the 1st and 3rd quartiles.}
\label{Fig:Loss}
\end{figure}

\begin{figure}[h]
\includegraphics[trim={0 0 0 0},clip,width=\columnwidth]{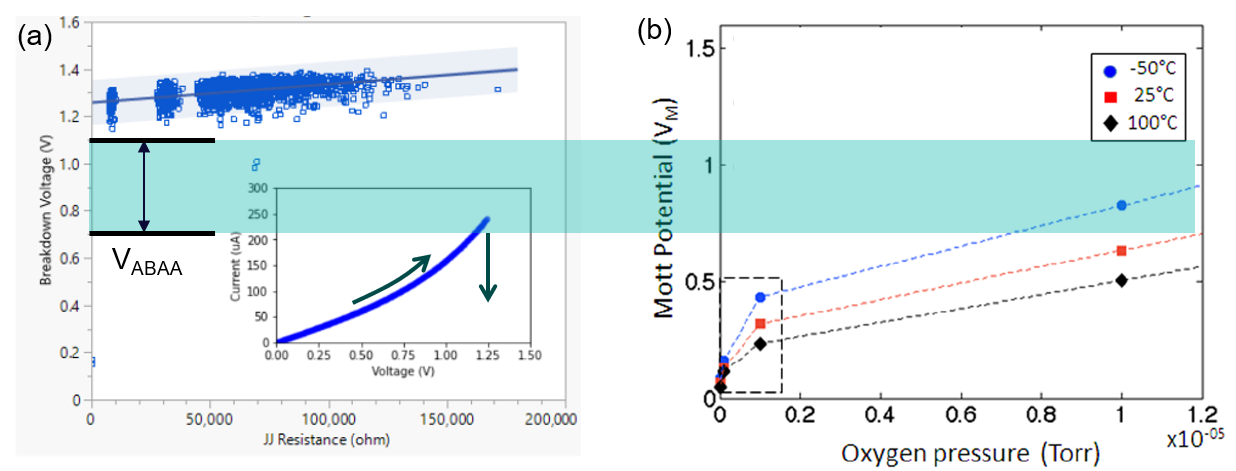}
  \caption{\\
  Title: Method to find the operational voltage range for ABAA\\
  Legend: Panel (a) Measured breakdown voltages as a function of junction resistance for large ensemble of junctions, inset - typical IV-curve of a single junction to breakdown. The voltage range for $V_{ABAA}$ for these junctions in the range of 5-50 k$\ohm$ is indicated as well, where it is greater than the Mott Potential at 25 $\degree$C, but less than the breakdown voltage.\\
  Panel (b) Data from Ref.~\cite{TemperatureAndPressureMottPotentials2012} showing the Mott voltage developed at the Al surface during oxidation at various temperatures.}
\label{Fig:ABAA_Voltage_Range}
\end{figure}
\newpage
\clearpage
\onecolumngrid{}
\section*{Supplementary References}
\printbibliography[heading=none]
\end{document}
